# Supplementary material for: Biomimetic non-ergodic aging by dynamic-to-covalent transitions in physical hydrogels
Source: arXiv:2311.15067 source file (2023-11-25)
Supplement: Supplementary file 1 [file SI_PDF.pdf]

# Supplementary Information

## Biomimetic non-ergodic aging by dynamic-to-covalent transitions in physical hydrogels

Samya Sen[1], Anthony C. Yu[1], Changxin Dong[1], Andrea I. D'Aquino[1], and Eric A. Appel*[1,2,3,4,5,6]

[1] *Department of Materials Science & Engineering, Stanford University, Stanford, CA 94305, USA*
[2] *Department of Bioengineering, Stanford University, Stanford, CA 94305, USA*
[3] *Stanford ChEM-H, Stanford University, Stanford, CA 94305, USA*
[4] *Institute for Immunity, Transplantation and Infection, Stanford University School of Medicine, Stanford, CA 94305, USA*
[5] *Department of Pediatrics - Endocrinology, Stanford University School of Medicine, Stanford, CA 94305, USA*
[6] *Woods Institute for the Environment, Stanford University, Stanford CA 94305, USA*

*Corresponding author: eappel@stanford.edu

# 1 Tuning aging by varying cellulose derivatives architecture

In the paper, we discussed methods for tuning the entropic-to-enthalpic transition using temperature and $p$H. We also mentioned the possibility of achieving the same using a differently modified cellulose backbone. Instead of using a combination of hydroxyethylcellulose (HEC) and methylcellulose (MC) which have a significant fraction of dangling $-$OH groups on the sugar rings, ready to react with silanols on the CSP surface, we can use hydroxyethylmethylcellulose (HEMC) as the polymer. This cellulose variant has fewer free $-$OH groups available to participate in the condensation reaction, and hence age much slower. A comparison of aging rheology for a hydrogel system with CSP mixed with HEC-MC and HEMC respectively is shown in Fig. 1.

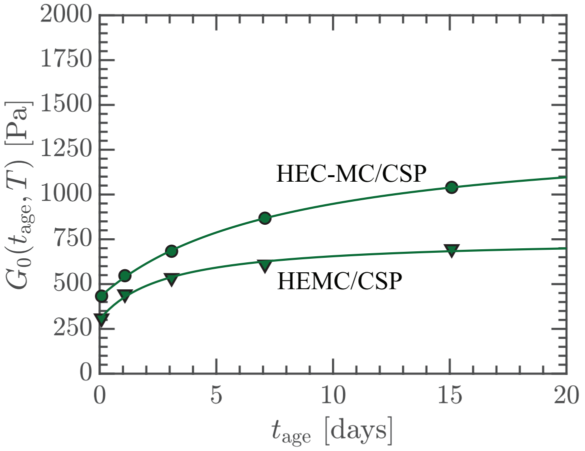


Figure 1: Aging in two hydrogel systems with different cellulose derivatives. HEC-MC/CSP ages faster than HEMC/CSP, and is hence softer. The fit lines are for the second order kinetic equation discussed in the paper.

The gels were prepared in $p$H 7 and stored at 25°C. We see that gels made with HEMC are softer than HEC-MC, as indicated by the modulus $G_0(t_{\mathrm{age}}, T)$. This is due to fewer reaction sites, and HEMC/CSP ages slower than HEC-MC/CSP hydrogels.

## 2 FTIR transmittance data

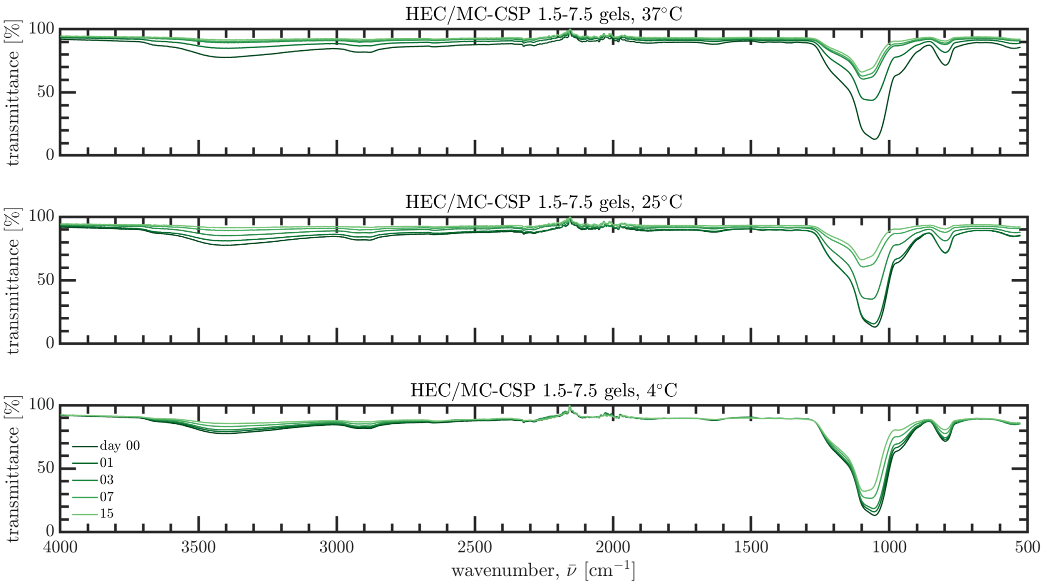


Figure 2: FTIR-ATR data for gels, showing the effect of temperature and age on transmittance spectrum.

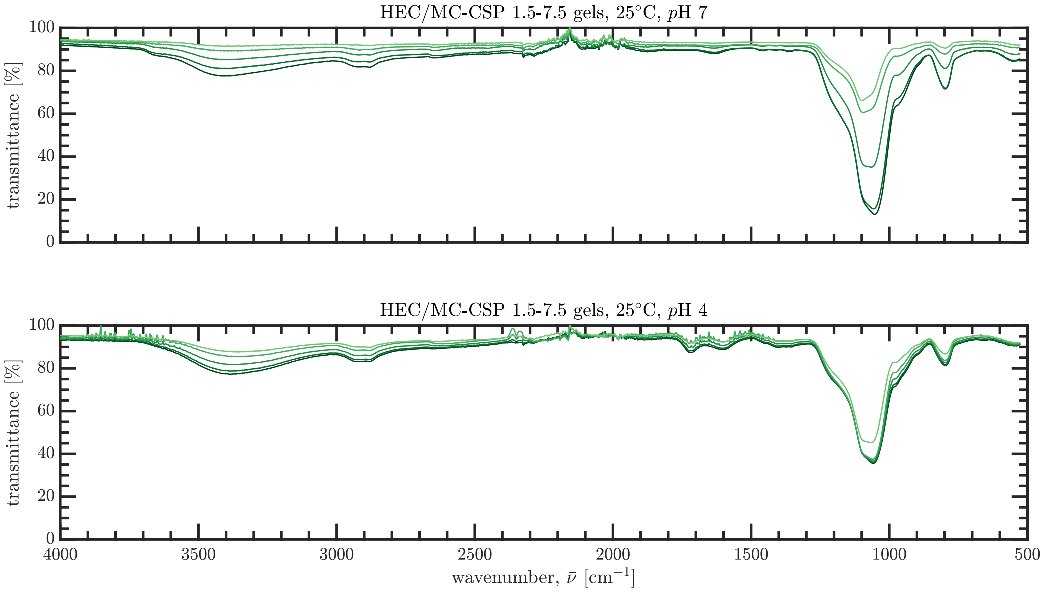


Figure 3: FTIR-ATR data for gels, showing the effect of *p*H and age on transmittance spectrum.

We have used absorbance data in the paper to quantify the aging process by monitoring the absorbance peak at 3410 cm$^{-1}$. Zooming in on the wavenumber range of 3200-3600 cm$^{-1}$, the effect of aging on the disappearance of $-$OH bonds was very clear. Here, we show the full range of FTIR data collected in terms of transmittance for wavenumbers 500-4000 cm$^{-1}$.

In Fig. 2, we see the effect of temperature, where the transmittance peak becomes weaker faster at elevated temperatures. In Fig. 3, we see the effect of $p$H, where the transmittance peak becomes weaker faster at higher $p$H. In both figures, also note the slow diminishing of the Si$-$OH peak at $\sim$ 1050 cm$^{-1}$. This effect goes hand-in-hand with the disappearance of the $-$OH peak as the material ages.
